# Supplementary material for: Grand Challenges around Designing Computers' Control Over Our Bodies
Source: arXiv:2601.19143 source file (2026-02-06)
Supplement: Supplementary file 1 [file appendix.tex]

\appendix

\section{Compiled Challenges}
We gathered 118 challenges from discussions and grouped them across themes such as method, technology, user, society, and design.
These subsequently were combined into the grand challenges described in Section~\ref{sec:GrandChallenges}.

\begin{enumerate}
\item \textbf{Entry:} Parasite, friend, part of me, \textbf{Final Label:} Parasite vs Assistant, \textbf{Our Interpretation:} N/A, \textbf{Method:} N/A, \textbf{Technology:} N/A, \textbf{User:} N/A, \textbf{Society:} N/A, \textbf{Design:} Parasite vs Assistant
\item \textbf{Entry:} How should it be designed to allow integration (rather than a parasite an assistant into your body/mind), \textbf{Final Label:} Parasite vs Assistant, \textbf{Our Interpretation:} N/A, \textbf{Method:} N/A, \textbf{Technology:} N/A, \textbf{User:} N/A, \textbf{Society:} N/A, \textbf{Design:} Parasite vs Assistant
\item \textbf{Entry:} Laziness, \textbf{Final Label:} Laziness, \textbf{Our Interpretation:} N/A, \textbf{Method:} N/A, \textbf{Technology:} N/A, \textbf{User:} Laziness, \textbf{Society:} N/A, \textbf{Design:} N/A
\item \textbf{Entry:} Spaces of control, \textbf{Final Label:} Spaces of control, \textbf{Our Interpretation:} N/A, \textbf{Method:} N/A, \textbf{Technology:} N/A, \textbf{User:} N/A, \textbf{Society:} Spaces of control, \textbf{Design:} N/A
\item \textbf{Entry:} Computer-initiated vs Human/Body Initiated, \textbf{Final Label:} Initiative, \textbf{Our Interpretation:} N/A, \textbf{Method:} N/A, \textbf{Technology:} N/A, \textbf{User:} N/A, \textbf{Society:} N/A, \textbf{Design:} Initiative
\item \textbf{Entry:} Implicit control \textless{}=\textgreater Explicit control, \textbf{Final Label:} Implicit vs Explicit, \textbf{Our Interpretation:} N/A, \textbf{Method:} N/A, \textbf{Technology:} N/A, \textbf{User:} N/A, \textbf{Society:} N/A, \textbf{Design:} Implicit vs Explicit
\item \textbf{Entry:} Belifes about capability/competence, \textbf{Final Label:} Belief of competence, \textbf{Our Interpretation:} N/A, \textbf{Method:} N/A, \textbf{Technology:} N/A, \textbf{User:} Belief of competence, \textbf{Society:} N/A, \textbf{Design:} N/A
\item \textbf{Entry:} Sense of agency vs Feeling of agency, \textbf{Final Label:} Agency, \textbf{Our Interpretation:} N/A, \textbf{Method:} N/A, \textbf{Technology:} N/A, \textbf{User:} N/A, \textbf{Society:} N/A, \textbf{Design:} Agency
\item \textbf{Entry:} Inattentional/attentional action binding, \textbf{Final Label:} Measurement of sense of agency, \textbf{Our Interpretation:} N/A, \textbf{Method:} Measurement of sense of agency, \textbf{Technology:} N/A, \textbf{User:} N/A, \textbf{Society:} N/A, \textbf{Design:} N/A
\item \textbf{Entry:} Body as Canvas + Social environment cultural values, \textbf{Final Label:} Social environment and cultural valuesBody as canvas, \textbf{Our Interpretation:} N/A, \textbf{Method:} N/A, \textbf{Technology:} N/A, \textbf{User:} N/A, \textbf{Society:} Social environment and cultural values, \textbf{Design:} Body as canvas
\item \textbf{Entry:} Safety, feeling safe and comfortable. No unpleasant suprises, \textbf{Final Label:} Feeling of safety. Comfort.Communcating system's intentions, \textbf{Our Interpretation:} N/A, \textbf{Method:} N/A, \textbf{Technology:} N/A, \textbf{User:} Feeling of safety. Comfort., \textbf{Society:} N/A, \textbf{Design:} Communcating system's intentions
\item \textbf{Entry:} Control \textless{}=\textgreater Agency, \textbf{Final Label:} Control vs. Agency, \textbf{Our Interpretation:} N/A, \textbf{Method:} N/A, \textbf{Technology:} N/A, \textbf{User:} N/A, \textbf{Society:} N/A, \textbf{Design:} Control vs. Agency
\item \textbf{Entry:} Control-change tradeoff (is not zero-sum), \textbf{Final Label:} Transfer of control, \textbf{Our Interpretation:} N/A, \textbf{Method:} N/A, \textbf{Technology:} N/A, \textbf{User:} N/A, \textbf{Society:} N/A, \textbf{Design:} Transfer of control
\item \textbf{Entry:} Transparency/Informed transfer of control, \textbf{Final Label:} Informed transfer of control, \textbf{Our Interpretation:} N/A, \textbf{Method:} N/A, \textbf{Technology:} N/A, \textbf{User:} N/A, \textbf{Society:} N/A, \textbf{Design:} Informed transfer of control
\item \textbf{Entry:} Surrendering/ giving up/losing control, \textbf{Final Label:} Transfer of control, \textbf{Our Interpretation:} N/A, \textbf{Method:} N/A, \textbf{Technology:} N/A, \textbf{User:} N/A, \textbf{Society:} N/A, \textbf{Design:} Transfer of control
\item \textbf{Entry:} Relation with augmented technology using Play Theory (4 play types), \textbf{Final Label:} Play Theory, \textbf{Our Interpretation:} N/A, \textbf{Method:} N/A, \textbf{Technology:} N/A, \textbf{User:} N/A, \textbf{Society:} N/A, \textbf{Design:} Play Theory
\item \textbf{Entry:} Persuasion, \textbf{Final Label:} Transfer of control, \textbf{Our Interpretation:} N/A, \textbf{Method:} N/A, \textbf{Technology:} N/A, \textbf{User:} N/A, \textbf{Society:} N/A, \textbf{Design:} Transfer of control
\item \textbf{Entry:} Regain control, \textbf{Final Label:} Transfer of control, \textbf{Our Interpretation:} N/A, \textbf{Method:} N/A, \textbf{Technology:} N/A, \textbf{User:} N/A, \textbf{Society:} N/A, \textbf{Design:} Transfer of control
\item \textbf{Entry:} Level of personalization and individual preferences, \textbf{Final Label:} Personalization and Customization, \textbf{Our Interpretation:} N/A, \textbf{Method:} N/A, \textbf{Technology:} N/A, \textbf{User:} Personalization and Customization, \textbf{Society:} N/A, \textbf{Design:} N/A
\item \textbf{Entry:} Level of automation and sense of agency, \textbf{Final Label:} Automation vs Agency, \textbf{Our Interpretation:} N/A, \textbf{Method:} N/A, \textbf{Technology:} N/A, \textbf{User:} N/A, \textbf{Society:} N/A, \textbf{Design:} Automation vs Agency
\item \textbf{Entry:} Signals, entrypoints, targets, \textbf{Final Label:} Design space, \textbf{Our Interpretation:} N/A, \textbf{Method:} N/A, \textbf{Technology:} N/A, \textbf{User:} N/A, \textbf{Society:} N/A, \textbf{Design:} Design space
\item \textbf{Entry:} Signal intensity vs User disposition to obey, \textbf{Final Label:} Control signal intensityUser obedience, \textbf{Our Interpretation:} N/A, \textbf{Method:} N/A, \textbf{Technology:} Control signal intensity, \textbf{User:} User obedience, \textbf{Society:} N/A, \textbf{Design:} N/A
\item \textbf{Entry:} Lack of knowledge on responses of our body’s physiology to external stimulations, \textbf{Final Label:} Elicitated responses, \textbf{Our Interpretation:} N/A, \textbf{Method:} N/A, \textbf{Technology:} Elicitated responses, \textbf{User:} N/A, \textbf{Society:} N/A, \textbf{Design:} N/A
\item \textbf{Entry:} Ethical challenges, \textbf{Final Label:} Ethics, \textbf{Our Interpretation:} N/A, \textbf{Method:} N/A, \textbf{Technology:} N/A, \textbf{User:} N/A, \textbf{Society:} Ethics, \textbf{Design:} N/A
\item \textbf{Entry:} Who is in control?, \textbf{Final Label:} Ownership of control, \textbf{Our Interpretation:} N/A, \textbf{Method:} N/A, \textbf{Technology:} N/A, \textbf{User:} N/A, \textbf{Society:} N/A, \textbf{Design:} Ownership of control
\item \textbf{Entry:} adaptation versus adoption between humans and computers – and their experiential implications, \textbf{Final Label:} Adaptation vs Adoption, \textbf{Our Interpretation:} N/A, \textbf{Method:} N/A, \textbf{Technology:} N/A, \textbf{User:} N/A, \textbf{Society:} N/A, \textbf{Design:} Adaptation vs Adoption
\item \textbf{Entry:} Computer-Supported Control over Body (CSCB), \textbf{Final Label:} CSCB, \textbf{Our Interpretation:} N/A, \textbf{Method:} N/A, \textbf{Technology:} N/A, \textbf{User:} N/A, \textbf{Society:} N/A, \textbf{Design:} CSCB
\item \textbf{Entry:} Explainable and transparent intervention approaches, \textbf{Final Label:} Explainability and Transparency, \textbf{Our Interpretation:} N/A, \textbf{Method:} N/A, \textbf{Technology:} N/A, \textbf{User:} N/A, \textbf{Society:} N/A, \textbf{Design:} Explainability and Transparency
\item \textbf{Entry:} What is our sun? Try to identify the extent of symbiosis/integration/manipulation., \textbf{Final Label:} Limits of control, \textbf{Our Interpretation:} N/A, \textbf{Method:} N/A, \textbf{Technology:} N/A, \textbf{User:} N/A, \textbf{Society:} N/A, \textbf{Design:} Limits of control
\item \textbf{Entry:} What scenarios or applications should we build for?, \textbf{Final Label:} Applications, \textbf{Our Interpretation:} N/A, \textbf{Method:} N/A, \textbf{Technology:} N/A, \textbf{User:} N/A, \textbf{Society:} N/A, \textbf{Design:} Applications
\item \textbf{Entry:} How does the computer understand what it can control?, \textbf{Final Label:} Control representation, \textbf{Our Interpretation:} N/A, \textbf{Method:} N/A, \textbf{Technology:} Control representation, \textbf{User:} N/A, \textbf{Society:} N/A, \textbf{Design:} N/A
\item \textbf{Entry:} Redirection is fun. But its really interesting in multi-user systems. What I am doing and what you see can be entirely different. How do I control this? What does this control mean for trust?, \textbf{Final Label:} Trust, \textbf{Our Interpretation:} N/A, \textbf{Method:} N/A, \textbf{Technology:} N/A, \textbf{User:} Trust, \textbf{Society:} N/A, \textbf{Design:} N/A
\item \textbf{Entry:} Can we benchmark control?, \textbf{Final Label:} Benchmark, \textbf{Our Interpretation:} N/A, \textbf{Method:} Benchmark, \textbf{Technology:} N/A, \textbf{User:} N/A, \textbf{Society:} N/A, \textbf{Design:} N/A
\item \textbf{Entry:} Do we understand Control well enough to think about Control in Augmentation Systems?, \textbf{Final Label:} Concept of control, \textbf{Our Interpretation:} N/A, \textbf{Method:} N/A, \textbf{Technology:} N/A, \textbf{User:} N/A, \textbf{Society:} N/A, \textbf{Design:} Concept of control
\item \textbf{Entry:} Definition of Control, \textbf{Final Label:} Concept of control, \textbf{Our Interpretation:} N/A, \textbf{Method:} N/A, \textbf{Technology:} N/A, \textbf{User:} N/A, \textbf{Society:} N/A, \textbf{Design:} Concept of control
\item \textbf{Entry:} Defining control, shared control, augmentation, intervention, \textbf{Final Label:} Concept of control, \textbf{Our Interpretation:} N/A, \textbf{Method:} N/A, \textbf{Technology:} N/A, \textbf{User:} N/A, \textbf{Society:} N/A, \textbf{Design:} Concept of control
\item \textbf{Entry:} Co-control, \textbf{Final Label:} Concept of control, \textbf{Our Interpretation:} N/A, \textbf{Method:} N/A, \textbf{Technology:} N/A, \textbf{User:} N/A, \textbf{Society:} N/A, \textbf{Design:} Concept of control
\item \textbf{Entry:} Impact of loss of control (e.g., facial paralysis leads to loss of control, cannot talk/chew/emote as desired)., \textbf{Final Label:} Concept of control, \textbf{Our Interpretation:} N/A, \textbf{Method:} N/A, \textbf{Technology:} N/A, \textbf{User:} N/A, \textbf{Society:} N/A, \textbf{Design:} Concept of control
\item \textbf{Entry:} How does loss of sense of body impact what control means (e.g., prosthetics)., \textbf{Final Label:} Concept of control, \textbf{Our Interpretation:} N/A, \textbf{Method:} N/A, \textbf{Technology:} N/A, \textbf{User:} N/A, \textbf{Society:} N/A, \textbf{Design:} Concept of control
\item \textbf{Entry:} What do we mean when we say the computer has “control” over one's body?, \textbf{Final Label:} Concept of control, \textbf{Our Interpretation:} N/A, \textbf{Method:} N/A, \textbf{Technology:} N/A, \textbf{User:} N/A, \textbf{Society:} N/A, \textbf{Design:} Concept of control
\item \textbf{Entry:} What do we mean by the body?, \textbf{Final Label:} Concept of control, \textbf{Our Interpretation:} N/A, \textbf{Method:} N/A, \textbf{Technology:} N/A, \textbf{User:} N/A, \textbf{Society:} N/A, \textbf{Design:} Concept of control
\item \textbf{Entry:} Location (space), \textbf{Final Label:} Concept of control, \textbf{Our Interpretation:} N/A, \textbf{Method:} N/A, \textbf{Technology:} N/A, \textbf{User:} N/A, \textbf{Society:} N/A, \textbf{Design:} Concept of control
\item \textbf{Entry:} Location (body), \textbf{Final Label:} Concept of control, \textbf{Our Interpretation:} N/A, \textbf{Method:} N/A, \textbf{Technology:} N/A, \textbf{User:} N/A, \textbf{Society:} N/A, \textbf{Design:} Concept of control
\item \textbf{Entry:} What is the non-invasive EMG \textless{}\textgreater EMS equivalent for ?? \textless{}\textgreater GVS, \textbf{Final Label:} Concept of control, \textbf{Our Interpretation:} N/A, \textbf{Method:} N/A, \textbf{Technology:} N/A, \textbf{User:} N/A, \textbf{Society:} N/A, \textbf{Design:} Concept of control
\item \textbf{Entry:} Is the goal to train the body or is the tech always going to be needed., \textbf{Final Label:} Concept of control, \textbf{Our Interpretation:} N/A, \textbf{Method:} N/A, \textbf{Technology:} N/A, \textbf{User:} N/A, \textbf{Society:} N/A, \textbf{Design:} Concept of control
\item \textbf{Entry:} Computer Supported Control over Body, \textbf{Final Label:} Concept of control, \textbf{Our Interpretation:} N/A, \textbf{Method:} N/A, \textbf{Technology:} N/A, \textbf{User:} N/A, \textbf{Society:} N/A, \textbf{Design:} Concept of control
\item \textbf{Entry:} What are the most pressing real world applications, \textbf{Final Label:} Applications, \textbf{Our Interpretation:} N/A, \textbf{Method:} N/A, \textbf{Technology:} N/A, \textbf{User:} N/A, \textbf{Society:} N/A, \textbf{Design:} Applications
\item \textbf{Entry:} Voluntarily giving up control $\sim$social contract theory, \textbf{Final Label:} Transfer of control, \textbf{Our Interpretation:} N/A, \textbf{Method:} N/A, \textbf{Technology:} N/A, \textbf{User:} N/A, \textbf{Society:} N/A, \textbf{Design:} Transfer of control
\item \textbf{Entry:} Zero-sum game? Giving up control and taking back maybe give up one thing and get back something else, \textbf{Final Label:} Transfer of control, \textbf{Our Interpretation:} N/A, \textbf{Method:} N/A, \textbf{Technology:} N/A, \textbf{User:} N/A, \textbf{Society:} N/A, \textbf{Design:} Transfer of control
\item \textbf{Entry:} Freedom, \textbf{Final Label:} Transfer of control, \textbf{Our Interpretation:} N/A, \textbf{Method:} N/A, \textbf{Technology:} N/A, \textbf{User:} N/A, \textbf{Society:} N/A, \textbf{Design:} Transfer of control
\item \textbf{Entry:} Power relationships (social), \textbf{Final Label:} came from conversation on what does control mean in a social setting Transfer of control, \textbf{Our Interpretation:} came from conversation on what does control mean in a social setting, \textbf{Method:} N/A, \textbf{Technology:} N/A, \textbf{User:} N/A, \textbf{Society:} N/A, \textbf{Design:} Transfer of control
\item \textbf{Entry:} Culture - that "computer/machine" is coming close to my body - how do I like that? I would not let anyone touch my shadow!, \textbf{Final Label:} Transfer of control, \textbf{Our Interpretation:} N/A, \textbf{Method:} N/A, \textbf{Technology:} N/A, \textbf{User:} N/A, \textbf{Society:} N/A, \textbf{Design:} Transfer of control
\item \textbf{Entry:} Intentionality vs relationality, \textbf{Final Label:} Trade-offs, \textbf{Our Interpretation:} N/A, \textbf{Method:} N/A, \textbf{Technology:} N/A, \textbf{User:} N/A, \textbf{Society:} N/A, \textbf{Design:} Trade-offs
\item \textbf{Entry:} Scale vs hierarchy, \textbf{Final Label:} Came out of conversation about telling a 3d printer what to print and the printer performing that task with no volitionTrade-offs, \textbf{Our Interpretation:} Came out of conversation about telling a 3d printer what to print and the printer performing that task with no volition, \textbf{Method:} N/A, \textbf{Technology:} N/A, \textbf{User:} N/A, \textbf{Society:} N/A, \textbf{Design:} Trade-offs
\item \textbf{Entry:} Macro vs micro goals, \textbf{Final Label:} Trade-offs, \textbf{Our Interpretation:} N/A, \textbf{Method:} N/A, \textbf{Technology:} N/A, \textbf{User:} N/A, \textbf{Society:} N/A, \textbf{Design:} Trade-offs
\item \textbf{Entry:} Interface vs control, \textbf{Final Label:} Trade-offs, \textbf{Our Interpretation:} N/A, \textbf{Method:} N/A, \textbf{Technology:} N/A, \textbf{User:} N/A, \textbf{Society:} N/A, \textbf{Design:} Trade-offs
\item \textbf{Entry:} Body vs mind, \textbf{Final Label:} Trade-offs, \textbf{Our Interpretation:} N/A, \textbf{Method:} N/A, \textbf{Technology:} N/A, \textbf{User:} N/A, \textbf{Society:} N/A, \textbf{Design:} Trade-offs
\item \textbf{Entry:} Does control over the human body mean to control body and mind?, \textbf{Final Label:} Trade-offs, \textbf{Our Interpretation:} N/A, \textbf{Method:} N/A, \textbf{Technology:} N/A, \textbf{User:} N/A, \textbf{Society:} N/A, \textbf{Design:} Trade-offs
\item \textbf{Entry:} Augmentation vs control, \textbf{Final Label:} Trade-offs, \textbf{Our Interpretation:} N/A, \textbf{Method:} N/A, \textbf{Technology:} N/A, \textbf{User:} N/A, \textbf{Society:} N/A, \textbf{Design:} Trade-offs
\item \textbf{Entry:} Sense of agency vs feeling of agency, \textbf{Final Label:} Trade-offs, \textbf{Our Interpretation:} N/A, \textbf{Method:} N/A, \textbf{Technology:} N/A, \textbf{User:} N/A, \textbf{Society:} N/A, \textbf{Design:} Trade-offs
\item \textbf{Entry:} Long-term control device vs in-lab/short term, \textbf{Final Label:} Trade-offs, \textbf{Our Interpretation:} N/A, \textbf{Method:} N/A, \textbf{Technology:} N/A, \textbf{User:} N/A, \textbf{Society:} N/A, \textbf{Design:} Trade-offs
\item \textbf{Entry:} Wearable vs environmental, \textbf{Final Label:} Trade-offs, \textbf{Our Interpretation:} N/A, \textbf{Method:} N/A, \textbf{Technology:} N/A, \textbf{User:} N/A, \textbf{Society:} N/A, \textbf{Design:} Trade-offs
\item \textbf{Entry:} Dystopian vs utopian, \textbf{Final Label:} Trade-offs, \textbf{Our Interpretation:} N/A, \textbf{Method:} N/A, \textbf{Technology:} N/A, \textbf{User:} N/A, \textbf{Society:} N/A, \textbf{Design:} Trade-offs
\item \textbf{Entry:} Choice vs not - who is deciding, \textbf{Final Label:} Trade-offs, \textbf{Our Interpretation:} N/A, \textbf{Method:} N/A, \textbf{Technology:} N/A, \textbf{User:} N/A, \textbf{Society:} N/A, \textbf{Design:} Trade-offs
\item \textbf{Entry:} Trade-off between agency and automation, \textbf{Final Label:} Trade-offs, \textbf{Our Interpretation:} N/A, \textbf{Method:} N/A, \textbf{Technology:} N/A, \textbf{User:} N/A, \textbf{Society:} N/A, \textbf{Design:} Trade-offs
\item \textbf{Entry:} Assist/augment/replace, \textbf{Final Label:} Trade-offs, \textbf{Our Interpretation:} N/A, \textbf{Method:} N/A, \textbf{Technology:} N/A, \textbf{User:} N/A, \textbf{Society:} N/A, \textbf{Design:} Trade-offs
\item \textbf{Entry:} Do we mean to help, to augment or to replace human behavior?, \textbf{Final Label:} Trade-offs, \textbf{Our Interpretation:} N/A, \textbf{Method:} N/A, \textbf{Technology:} N/A, \textbf{User:} N/A, \textbf{Society:} N/A, \textbf{Design:} Trade-offs
\item \textbf{Entry:} Transcendent responsibility, \textbf{Final Label:} Trade-offs, \textbf{Our Interpretation:} N/A, \textbf{Method:} N/A, \textbf{Technology:} N/A, \textbf{User:} N/A, \textbf{Society:} N/A, \textbf{Design:} Trade-offs
\item \textbf{Entry:} Calibration, \textbf{Final Label:} came from conversation about GVS needing to be personalizedTechnology, \textbf{Our Interpretation:} came from conversation about GVS needing to be personalized, \textbf{Method:} N/A, \textbf{Technology:} Technology, \textbf{User:} N/A, \textbf{Society:} N/A, \textbf{Design:} N/A
\item \textbf{Entry:} Reading and writing GVS signals, \textbf{Final Label:} Technology, \textbf{Our Interpretation:} N/A, \textbf{Method:} N/A, \textbf{Technology:} Technology, \textbf{User:} N/A, \textbf{Society:} N/A, \textbf{Design:} N/A
\item \textbf{Entry:} Quantify impact of aging on the senses, \textbf{Final Label:} Adoption, \textbf{Our Interpretation:} N/A, \textbf{Method:} N/A, \textbf{Technology:} N/A, \textbf{User:} Adoption, \textbf{Society:} N/A, \textbf{Design:} N/A
\item \textbf{Entry:} Interaction, \textbf{Final Label:} Interaction, \textbf{Our Interpretation:} N/A, \textbf{Method:} N/A, \textbf{Technology:} N/A, \textbf{User:} Interaction, \textbf{Society:} N/A, \textbf{Design:} N/A
\item \textbf{Entry:} (Inter)action outcome, \textbf{Final Label:} Interaction, \textbf{Our Interpretation:} N/A, \textbf{Method:} N/A, \textbf{Technology:} N/A, \textbf{User:} Interaction, \textbf{Society:} N/A, \textbf{Design:} N/A
\item \textbf{Entry:} Temporal scale of control, \textbf{Final Label:} Interaction, \textbf{Our Interpretation:} N/A, \textbf{Method:} N/A, \textbf{Technology:} N/A, \textbf{User:} Interaction, \textbf{Society:} N/A, \textbf{Design:} N/A
\item \textbf{Entry:} Implications for long-term use, \textbf{Final Label:} Adoption, \textbf{Our Interpretation:} N/A, \textbf{Method:} N/A, \textbf{Technology:} N/A, \textbf{User:} Adoption, \textbf{Society:} N/A, \textbf{Design:} N/A
\item \textbf{Entry:} Time (duration, frequency), \textbf{Final Label:} Interaction, \textbf{Our Interpretation:} N/A, \textbf{Method:} N/A, \textbf{Technology:} N/A, \textbf{User:} Interaction, \textbf{Society:} N/A, \textbf{Design:} N/A
\item \textbf{Entry:} Methods for understanding control, \textbf{Final Label:} Understanding controlBacking Theory, \textbf{Our Interpretation:} N/A, \textbf{Method:} Understanding control, \textbf{Technology:} N/A, \textbf{User:} N/A, \textbf{Society:} N/A, \textbf{Design:} Backing Theory
\item \textbf{Entry:} SDT \textless{}\textgreater control, \textbf{Final Label:} self determination theoryBacking Theory, \textbf{Our Interpretation:} self determination theory, \textbf{Method:} N/A, \textbf{Technology:} N/A, \textbf{User:} N/A, \textbf{Society:} N/A, \textbf{Design:} Backing Theory
\item \textbf{Entry:} Placebo - visual augmentations to face/body, \textbf{Final Label:} came out of conversation about adding bunny ears to face and if that can lead to an identity over time and if that identity has an impact on behavior \textgreater proteus effect or on self-perception \textgreater placebo effect (e.g., looking younger facial filter)User-centric, \textbf{Our Interpretation:} came out of conversation about adding bunny ears to face and if that can lead to an identity over time and if that identity has an impact on behavior \textgreater proteus effect or on self-perception \textgreater placebo effect (e.g., looking younger facial filter), \textbf{Method:} N/A, \textbf{Technology:} N/A, \textbf{User:} User-centric, \textbf{Society:} N/A, \textbf{Design:} N/A
\item \textbf{Entry:} Proteus effect, \textbf{Final Label:} User-centric, \textbf{Our Interpretation:} N/A, \textbf{Method:} N/A, \textbf{Technology:} N/A, \textbf{User:} User-centric, \textbf{Society:} N/A, \textbf{Design:} N/A
\item \textbf{Entry:} Effect on perception of self, \textbf{Final Label:} User-centric, \textbf{Our Interpretation:} N/A, \textbf{Method:} N/A, \textbf{Technology:} N/A, \textbf{User:} User-centric, \textbf{Society:} N/A, \textbf{Design:} N/A
\item \textbf{Entry:} Level of personalization, \textbf{Final Label:} User-centric, \textbf{Our Interpretation:} N/A, \textbf{Method:} N/A, \textbf{Technology:} N/A, \textbf{User:} User-centric, \textbf{Society:} N/A, \textbf{Design:} N/A
\item \textbf{Entry:} Personalized continuum, \textbf{Final Label:} User-centric, \textbf{Our Interpretation:} N/A, \textbf{Method:} N/A, \textbf{Technology:} N/A, \textbf{User:} User-centric, \textbf{Society:} N/A, \textbf{Design:} N/A
\item \textbf{Entry:} Perception, \textbf{Final Label:} User-centric, \textbf{Our Interpretation:} N/A, \textbf{Method:} N/A, \textbf{Technology:} N/A, \textbf{User:} User-centric, \textbf{Society:} N/A, \textbf{Design:} N/A
\item \textbf{Entry:} Experience, \textbf{Final Label:} User-centric, \textbf{Our Interpretation:} N/A, \textbf{Method:} N/A, \textbf{Technology:} N/A, \textbf{User:} User-centric, \textbf{Society:} N/A, \textbf{Design:} N/A
\item \textbf{Entry:} Explainable intervention, \textbf{Final Label:} Communicating and Signalling Control, \textbf{Our Interpretation:} N/A, \textbf{Method:} N/A, \textbf{Technology:} N/A, \textbf{User:} N/A, \textbf{Society:} N/A, \textbf{Design:} Communicating and Signalling Control
\item \textbf{Entry:} Intentionality transparency, \textbf{Final Label:} Communicating and Signalling Control, \textbf{Our Interpretation:} N/A, \textbf{Method:} N/A, \textbf{Technology:} N/A, \textbf{User:} N/A, \textbf{Society:} N/A, \textbf{Design:} Communicating and Signalling Control
\item \textbf{Entry:} (How) do we make control transparent to the user?, \textbf{Final Label:} Communicating and Signalling Control, \textbf{Our Interpretation:} N/A, \textbf{Method:} N/A, \textbf{Technology:} N/A, \textbf{User:} N/A, \textbf{Society:} N/A, \textbf{Design:} Communicating and Signalling Control
\item \textbf{Entry:} Lack of knowledge of mechanism, \textbf{Final Label:} Communicating and Signalling Control, \textbf{Our Interpretation:} N/A, \textbf{Method:} N/A, \textbf{Technology:} N/A, \textbf{User:} N/A, \textbf{Society:} N/A, \textbf{Design:} Communicating and Signalling Control
\item \textbf{Entry:} Visibility, \textbf{Final Label:} Communicating and Signalling Control, \textbf{Our Interpretation:} N/A, \textbf{Method:} N/A, \textbf{Technology:} N/A, \textbf{User:} N/A, \textbf{Society:} N/A, \textbf{Design:} Communicating and Signalling Control
\item \textbf{Entry:} Awareness, \textbf{Final Label:} Communicating and Signalling Control, \textbf{Our Interpretation:} N/A, \textbf{Method:} N/A, \textbf{Technology:} N/A, \textbf{User:} N/A, \textbf{Society:} N/A, \textbf{Design:} Communicating and Signalling Control
\item \textbf{Entry:} Action, \textbf{Final Label:} Communicating and Signalling Control, \textbf{Our Interpretation:} N/A, \textbf{Method:} N/A, \textbf{Technology:} N/A, \textbf{User:} N/A, \textbf{Society:} N/A, \textbf{Design:} Communicating and Signalling Control
\item \textbf{Entry:} Anticipation, \textbf{Final Label:} Communicating and Signalling Control, \textbf{Our Interpretation:} N/A, \textbf{Method:} N/A, \textbf{Technology:} N/A, \textbf{User:} N/A, \textbf{Society:} N/A, \textbf{Design:} Communicating and Signalling Control
\item \textbf{Entry:} Getting users to trust systems to try, \textbf{Final Label:} Communicating and Signalling Control, \textbf{Our Interpretation:} N/A, \textbf{Method:} N/A, \textbf{Technology:} N/A, \textbf{User:} N/A, \textbf{Society:} N/A, \textbf{Design:} Communicating and Signalling Control
\item \textbf{Entry:} Familiarity/getting used to sensation, \textbf{Final Label:} Communicating and Signalling Control, \textbf{Our Interpretation:} N/A, \textbf{Method:} N/A, \textbf{Technology:} N/A, \textbf{User:} N/A, \textbf{Society:} N/A, \textbf{Design:} Communicating and Signalling Control
\item \textbf{Entry:} Can the human object to the control?, \textbf{Final Label:} Communicating and Signalling Control, \textbf{Our Interpretation:} N/A, \textbf{Method:} N/A, \textbf{Technology:} N/A, \textbf{User:} N/A, \textbf{Society:} N/A, \textbf{Design:} Communicating and Signalling Control
\item \textbf{Entry:} Do we plan to give control back to the human ?, \textbf{Final Label:} Communicating and Signalling Control, \textbf{Our Interpretation:} N/A, \textbf{Method:} N/A, \textbf{Technology:} N/A, \textbf{User:} N/A, \textbf{Society:} N/A, \textbf{Design:} Communicating and Signalling Control
\item \textbf{Entry:} Existential fusion, \textbf{Final Label:} Communicating and Signalling Control, \textbf{Our Interpretation:} N/A, \textbf{Method:} N/A, \textbf{Technology:} N/A, \textbf{User:} N/A, \textbf{Society:} N/A, \textbf{Design:} Communicating and Signalling Control
\item \textbf{Entry:} Body norms/accessibility/impairment/different bodies, \textbf{Final Label:} Acessibility, \textbf{Our Interpretation:} N/A, \textbf{Method:} N/A, \textbf{Technology:} N/A, \textbf{User:} N/A, \textbf{Society:} N/A, \textbf{Design:} Acessibility
\item \textbf{Entry:} Accessibility - who do we design for? Age?, \textbf{Final Label:} Acessibility, \textbf{Our Interpretation:} N/A, \textbf{Method:} N/A, \textbf{Technology:} N/A, \textbf{User:} N/A, \textbf{Society:} N/A, \textbf{Design:} Acessibility
\item \textbf{Entry:} Devices (progressively adaptive as the inner ear changes with age, exposure)., \textbf{Final Label:} Acessibility, \textbf{Our Interpretation:} N/A, \textbf{Method:} N/A, \textbf{Technology:} N/A, \textbf{User:} N/A, \textbf{Society:} N/A, \textbf{Design:} Acessibility
\item \textbf{Entry:} Level of support/control needed for novice vs. professional, \textbf{Final Label:} Acessibility, \textbf{Our Interpretation:} N/A, \textbf{Method:} N/A, \textbf{Technology:} N/A, \textbf{User:} N/A, \textbf{Society:} N/A, \textbf{Design:} Acessibility
\item \textbf{Entry:} Body manipulations (physically, can it take other forms?), \textbf{Final Label:} Modalities, \textbf{Our Interpretation:} N/A, \textbf{Method:} Modalities, \textbf{Technology:} N/A, \textbf{User:} N/A, \textbf{Society:} N/A, \textbf{Design:} N/A
\item \textbf{Entry:} Black mirror scenarios, \textbf{Final Label:} Imaginary scenario, \textbf{Our Interpretation:} N/A, \textbf{Method:} Imaginary scenario, \textbf{Technology:} N/A, \textbf{User:} N/A, \textbf{Society:} N/A, \textbf{Design:} N/A
\item \textbf{Entry:} Implicit vs Explicit / psych vs physical, \textbf{Final Label:} Trade-off, \textbf{Our Interpretation:} N/A, \textbf{Method:} N/A, \textbf{Technology:} N/A, \textbf{User:} N/A, \textbf{Society:} N/A, \textbf{Design:} Trade-off
\item \textbf{Entry:} Manipulation, \textbf{Final Label:} Manipulation, \textbf{Our Interpretation:} N/A, \textbf{Method:} N/A, \textbf{Technology:} N/A, \textbf{User:} N/A, \textbf{Society:} N/A, \textbf{Design:} Manipulation
\item \textbf{Entry:} Understanding of the body's relations to external structures, \textbf{Final Label:} Bodily understanding, \textbf{Our Interpretation:} N/A, \textbf{Method:} N/A, \textbf{Technology:} N/A, \textbf{User:} N/A, \textbf{Society:} N/A, \textbf{Design:} Bodily understanding
\item \textbf{Entry:} Granularity of control, \textbf{Final Label:} Granularity, \textbf{Our Interpretation:} N/A, \textbf{Method:} N/A, \textbf{Technology:} N/A, \textbf{User:} N/A, \textbf{Society:} N/A, \textbf{Design:} Granularity
\item \textbf{Entry:} How many wearables do we expect, \textbf{Final Label:} adoption of wearables, \textbf{Our Interpretation:} N/A, \textbf{Method:} N/A, \textbf{Technology:} N/A, \textbf{User:} adoption of wearables, \textbf{Society:} N/A, \textbf{Design:} N/A
\item \textbf{Entry:} Whole body vs components, \textbf{Final Label:} Body parts, \textbf{Our Interpretation:} N/A, \textbf{Method:} N/A, \textbf{Technology:} N/A, \textbf{User:} Body parts, \textbf{Society:} N/A, \textbf{Design:} N/A
\item \textbf{Entry:} Cultivate value ( feet), \textbf{Final Label:} Cultivate value, \textbf{Our Interpretation:} N/A, \textbf{Method:} N/A, \textbf{Technology:} N/A, \textbf{User:} N/A, \textbf{Society:} Cultivate value, \textbf{Design:} N/A
\item \textbf{Entry:} Intentionality, \textbf{Final Label:} N/A, \textbf{Our Interpretation:} N/A, \textbf{Method:} N/A, \textbf{Technology:} N/A, \textbf{User:} N/A, \textbf{Society:} N/A, \textbf{Design:} N/A
\item \textbf{Entry:} Are we having a reductionalist approach?, \textbf{Final Label:} N/A, \textbf{Our Interpretation:} N/A, \textbf{Method:} N/A, \textbf{Technology:} N/A, \textbf{User:} N/A, \textbf{Society:} N/A, \textbf{Design:} N/A
\item \textbf{Entry:} Who gets to design the system? Who has a say? I.e., who controls the design process or the computer?, \textbf{Final Label:} N/A, \textbf{Our Interpretation:} N/A, \textbf{Method:} N/A, \textbf{Technology:} N/A, \textbf{User:} N/A, \textbf{Society:} N/A, \textbf{Design:} N/A
\item \textbf{Entry:} How do we design the system to achieve the level of control?, \textbf{Final Label:} N/A, \textbf{Our Interpretation:} N/A, \textbf{Method:} N/A, \textbf{Technology:} N/A, \textbf{User:} N/A, \textbf{Society:} N/A, \textbf{Design:} N/A
\item \textbf{Entry:} Do we want to create dependency or create ability to be then learn to be in control?, \textbf{Final Label:} N/A, \textbf{Our Interpretation:} N/A, \textbf{Method:} N/A, \textbf{Technology:} N/A, \textbf{User:} N/A, \textbf{Society:} N/A, \textbf{Design:} N/A
\item \textbf{Entry:} Human changes at different timescales (not just long ones) and not always in the same directions (e.g., not always getting either better or worse), affective states induce temporary changes's in capabilities), \textbf{Final Label:} N/A, \textbf{Our Interpretation:} N/A, \textbf{Method:} N/A, \textbf{Technology:} N/A, \textbf{User:} N/A, \textbf{Society:} N/A, \textbf{Design:} N/A
\item \textbf{Entry:} Affective states alter perception and accepability etc., \textbf{Final Label:} N/A, \textbf{Our Interpretation:} N/A, \textbf{Method:} N/A, \textbf{Technology:} N/A, \textbf{User:} N/A, \textbf{Society:} N/A, \textbf{Design:} N/A
\end{enumerate}
